# Supplementary material for: Learning Robust Models for e-Commerce Product Search
Source: arXiv:2005.03624 source file (2020-05-07)
Supplement: Supplementary file 1 [file supp.tex]

% !TEX root = wsdm.tex

\onecolumn
\section{Supplemental Material}
\label{sec:supplemental}
